# Supplementary material for: Design Of a Dual-band Patch Antenna with Stacked Structure
Source: arXiv:2504.13609 source file (2025-04-18)
Supplement: Supplementary file 1 [file Appendix1.tex]

\documentclass[../Thesis]{subfiles}
\begin{document}

\chapter{This is an appendix}
\chaptermark{working with appendices yes}
nothing

\end{document}
